# Supplementary material for: High harmonic generation in monolayer MoS2 controlled by resonant and near-resonant pulses on ultrashort time scales
Source: arXiv:2504.02567 ancillary file (2025-04-03)
Supplement: Supplementary file 1 [file Supplementary_material.pdf]

# Supplementary material: High harmonic generation in monolayer $MoS_2$ controlled by resonant and near-resonant pulses on ultrashort time scales

Pavel Peterka,[†] Artur O. Slobodeniuk,[‡] Tomáš Novotný,[‡] Pawan Suthar,[†] Miroslav Bartoš,[¶] František Trojánek,[†] Petr Malý,[†] and Martin Kozák[*,†]

†*Department of Chemical Physics and Optics, Faculty of Mathematics and Physics, Charles University, Ke Karlovu 3, 12116 Prague 2, Czech Republic*

‡*Department of Condensed Matter Physics, Faculty of Mathematics and Physics, Charles University, Ke Karlovu 3, 12116 Prague 2, Czech Republic*

¶*Central European Institute of Technology, Brno University of Technology, Purkyňova 656/123, 612 00 Brno, Czech Republic*

E-mail: kozak@karlov.mff.cuni.cz

# 1 Theory of two-photon absorption in $MoS_2$ monolayer

## 1.1 Properties of the bands in TMD monolayer

We consider 7-band model of the TMD monolayer which goes beyond the simplest two-band case. The 7-band model contains 3 additional valence bands ($v-3$,$v-2$,$v-1$) below the valence ($v$) band and 2 conduction bands ($c+1$,$c+2$) above the conduction ($c$) one. We will focus on the bands' structure in the corners of the Brillouin zone of the TMD monolayer,

i.e. in $K^\pm$ points (valleys). For the sake of brevity we consider the properties of the bands in $K^+$ point. The analogous properties in $K^-$ point can be found with the help of time reversal symmetry operation, because both points transforms into each other by application of this symmetry.

The Bloch states in $K^+$ point of monolayer are $|\Psi_{v-3}, s\rangle$, $|\Psi_{v-2}, s\rangle$, $|\Psi_{v-1}, s\rangle$, $|\Psi_v, s\rangle$, $|\Psi_c, s\rangle$, $|\Psi_{c+1}, s\rangle$, $|\Psi_{c+2}, s\rangle$. The lower index $n = v-3, v-2, \dots c+1$ indicates the band, $s =\uparrow, \downarrow$ is the spin degree of freedom. The basis vectors are defined as a decomposition $|\Psi_n, s\rangle = |\Psi_n\rangle|s\rangle$. They can be classified according to irreducible representations of the symmetry group of the crystal.[1,2] All the group transformations are based on the in-plane $2\pi/3$ rotation $C_3$ and in-plane mirror reflection $\sigma_h$. The states $|\Psi_{v-3}, s\rangle$, $|\Psi_v, s\rangle$, $|\Psi_c, s\rangle$, $|\Psi_{c+2}, s\rangle$ are even under mirror transformation, while the $|\Psi_{v-2}, s\rangle$, $|\Psi_{v-1}, s\rangle$, $|\Psi_{c+1}, s\rangle$ are odd. The **kp** perturbation terms couple only the states with the same parity. Therefore we exclude the odd states from our consideration since they are not coupled to $v$ and $c$ bands, and therefore do not impact (as we see below) to the optical transitions between these bands.

Taking into account the transformation properties of the remaining states[3] $C_3|\Psi_v, s\rangle = |\Psi_v, s\rangle$, $C_3|\Psi_c, s\rangle = \omega^*|\Psi_c, s\rangle$, $C_3|\Psi_{v-3}, s\rangle = \omega|\Psi_{v-3}, s\rangle$, $C_3|\Psi_{c+2}, s\rangle = \omega|\Psi_{c+2}, s\rangle$ with $\omega = e^{2i\pi/3}$, one obtains **kp** matrix elements, presented in Table 1.[1,3,4] They form the **kp** part of

Table 1: **kp** matrix elements between the states with even parity of the monolayer.

| $H_{\mathbf{kp}}$ | $\|\Psi_v, s\rangle$ | $\|\Psi_c, s\rangle$ | $\|\Psi_{v-3}, s\rangle$ | $\|\Psi_{c+2}, s\rangle$ |
|---|---|---|---|---|
| $\|\Psi_v, s\rangle$ | $E_v$ | $\gamma_3 k_+$ | $\gamma_2 k_-$ | $\gamma_4 k_-$ |
| $\|\Psi_c, s\rangle$ | $\gamma_3^* k_-$ | $E_c$ | $\gamma_5 k_+$ | $\gamma_6 k_+$ |
| $\|\Psi_{v-3}, s\rangle$ | $\gamma_2^* k_+$ | $\gamma_5^* k_-$ | $E_{v-3}$ | 0 |
| $\|\Psi_{c+2}, s\rangle$ | $\gamma_4^* k_+$ | $\gamma_6^* k_-$ | 0 | $E_{c+2}$ |

the full single particle Hamiltonian, written in the basis of the corresponding Bloch states. For this matrix we introduced the notation $k_\pm = k_x \pm i k_y$. The set of the energies $\{E_n\}$ of

the corresponding states in $K^+$ point is written for clarity. They appear from the crystal field of the monolayer. The spin-orbit interaction, considered as a perturbation, gives the correction $\sigma_s \Delta_n/2$ to diagonal elements of the table, with $\sigma_s = +1(-1)$ for $\uparrow$ ($\downarrow$) states. The kinetic term of the electron gives also $\hbar^2 k^2/2m_0$ contribution to each diagonal element of this matrix. Here $m_0$ is an electron's mass.

The eigenstates of this matrix are the superposition of the basis states. Due to this superposition the several new channels of optical transitions are possible. For example the following two-photon induced processes are possible: $v \to c+2 \to c$, $v \to v-3 \to c$. Due to these processes the exciton, which has one hole in valence ($v$) band and an electron in conduction ($c$) band, is formed. This excitonic transition is happening via intermediate $c+2$ and $v-3$ bands. The other, more sophisticated, mechanisms of two-photon absorption can be found in Ref.[5]

## 1.2 Two-photon absorption: Fermi golden rule approach

The rate of optical transitions, induced simultaneously by two photons can be written as

$$\Gamma(f, in) = \frac{2\pi}{\hbar} |\langle f|U|in\rangle|^2 \delta(E_f - E_{in} - \hbar\omega_1 - \hbar\omega_2). \tag{1}$$

Here $\langle f|U|in\rangle$ is the matrix element of two-photon process. It couples the initial state $|in\rangle = |0\rangle$ (with occupied valence bands and empty conduction bands) and final exciton state $|f\rangle = |\mathbf{q}, n, \tau, c, v\rangle$ (with the total momentum $\mathbf{q}$, discrete quantum number $n$) consisting of an electron in conduction ($c$) band and a hole in valence ($v$) band of $\tau = \pm 1$ valley. We skip the bands' spin indices here, because optical transitions conserve spin, i.e., couples only the bands with the same spin. Here, the operator $U$ is responsible for the two-photon process. It corresponds to the second order processes in perturbation theory, see.[6,7] The perturbation operator is taken in the form $H_{\text{int}}(t) = -\mathbf{P} \cdot \mathbf{E}$, where $\mathbf{P}$ is the monolayer's polarization operator and $\mathbf{E}$ is the in-plane electric of incoming light pulses. Taking into account that

these pulses are linealy polarized with polarization vectors $\mathbf{e}_1$, $\mathbf{e}_2$, field amplitudes $|E_1|$, $|E_2|$, and phases $\phi_1$, $\phi_2$ we write

$$\begin{aligned}\mathbf{E} =&\mathbf{E}_1\cos(\omega_1 t+\phi_1)+\mathbf{E}_2\cos(\omega_2 t+\phi_2)=\\ =&(|E_1|e^{i\phi_1}e^{i\omega_1 t}+|E_1|e^{-i\phi_1}e^{-i\omega_1 t})\mathbf{e}_1+(|E_2|e^{i\phi_2}e^{i\omega_2 t}+|E_2|e^{-i\phi_2}e^{-i\omega_2 t})\mathbf{e}_2=\\ =&(E_1^*e^{i\omega_1 t}+E_1e^{-i\omega_1 t})\mathbf{e}_1+(E_2^*e^{i\omega_2 t}+E_2e^{-i\omega_2 t})\mathbf{e}_2.\end{aligned} \tag{2}$$

For this particular case the interaction term takes the form

$$H_{\text{int}}(t)=-\mathbf{P}\cdot\mathbf{e}_1(E_1^*e^{i\omega_1 t}+E_1e^{-i\omega_1 t})-\mathbf{P}\cdot\mathbf{e}_2(E_2^*e^{i\omega_2 t}+E_2e^{-i\omega_2 t}). \tag{3}$$

Using the results of Refs.[6,7] we obtain the following expression for the transition rate $\Gamma_{\mathbf{q}',m}$ to the excitonic state with energy $E_m(\mathbf{q}')$ due to two-photon absorption

$$\Gamma_{m,\mathbf{q}'}=\frac{2\pi}{\hbar}|E_1|^2|E_2|^2\Big[\sum_\tau|M_{\mathbf{q}',m,\tau}|^2\Big]\delta\big(E_m(\mathbf{q}')-\hbar[\omega_1+\omega_2]\big), \tag{4}$$

with the two-photon absorption amplitude

$$\begin{aligned}M_{\mathbf{q}',m,\tau}=\sum_\nu\Big[&\frac{\langle\mathbf{q}',m,\tau,c,v|(\mathbf{P}^\tau\cdot\mathbf{e}_1)|\nu\rangle\langle\nu|(\mathbf{P}^\tau\cdot\mathbf{e}_2)|0\rangle}{E_\nu-\hbar\omega_2}+\\ &+\frac{\langle\mathbf{q}',m,\tau,c,v|(\mathbf{P}^\tau\cdot\mathbf{e}_2)|\nu\rangle\langle\nu|(\mathbf{P}^\tau\cdot\mathbf{e}_1)|0\rangle}{E_\nu-\hbar\omega_1}\Big].\end{aligned} \tag{5}$$

Here, the index $\nu$ denote all the information about the excitonic states, i.e. $\nu=\mathbf{q},n,\tau,c+j,v-l$. Hence $E_\nu=E_n(\mathbf{q}')$ is the energy of the exciton in $\tau$ valley with momentum $\mathbf{q}$, quantum number $n$, consisting of an electron in $c+j$ $(j=0,1,\dots)$ conduction and a hole in $v-l$ $(l=0,1,\dots)$ valence bands, respectively. The polarization operator in a 7-band model can be written as a sum of interband terms

$$\mathbf{P}=\sum_\tau\mathbf{P}^\tau=\sum_\tau(\mathbf{P}^\tau_{c+2,v}+\mathbf{P}^\tau_{c,c+2}+\mathbf{P}^\tau_{c,v-3}+\mathbf{P}^\tau_{v,v-3}). \tag{6}$$

Using the matrix elements from the Tab. 1 and results of Ref.[8] we obtain

$$\mathbf{P}^{\tau}_{c+2,v} = -\frac{ie\tau}{(E_{c+2}-E_v)}\gamma_4^*(\mathbf{e}_x + i\mathbf{e}_y)\sum_{\mathbf{k}} a^{\dagger}_{\mathbf{k},c+2,\tau}a_{\mathbf{k},v,\tau} + \text{h.c.}, \tag{7}$$

$$\mathbf{P}^{\tau}_{c,c+2} = -\frac{ie\tau}{(E_{c+2}-E_c)}\gamma_6(\mathbf{e}_x + i\mathbf{e}_y)\sum_{\mathbf{k}} a^{\dagger}_{\mathbf{k},c,\tau}a_{\mathbf{k},c+2,\tau} + \text{h.c.}, \tag{8}$$

$$\mathbf{P}^{\tau}_{c,v-3} = -\frac{ie\tau}{(E_{c}-E_{v-3})}\gamma_5(\mathbf{e}_x + i\mathbf{e}_y)\sum_{\mathbf{k}} a^{\dagger}_{\mathbf{k},c,\tau}a_{\mathbf{k},v-3,\tau} + \text{h.c.}, \tag{9}$$

$$\mathbf{P}^{\tau}_{v,v-3} = -\frac{ie\tau}{(E_{v}-E_{v-3})}\gamma_2(\mathbf{e}_x - i\mathbf{e}_y)\sum_{\mathbf{k}} a^{\dagger}_{\mathbf{k},v,\tau}a_{\mathbf{k},v-3,\tau} + \text{h.c.}, \tag{10}$$

where $e$ is electron's charge, $\mathbf{e}_x$, $\mathbf{e}_y$ are in-plane unit orthogonal vectors. We introduced the annihilation operators $a_{\mathbf{k},v-l,\tau}$ and $a_{\mathbf{k},c+j,\tau}$, which destroy the electronic state with momentum $\mathbf{q}$, in the valley $\tau$ in the valence $(v-l)$ and the conduction $(c+j)$ bands, respectively. The analysis of $\mathbf{k}\cdot\mathbf{p}$ terms provides two different ways of two-photon transition. First way can be represented as by the set of virtual exciton transitions $|0\rangle \to |\mathbf{q}, n, \tau, c{+}2, v\rangle \to |\mathbf{q}', m, \tau, c, v\rangle$, while the second one is $|0\rangle \to |\mathbf{q}, n, \tau, c, v-3, \tau\rangle \to |\mathbf{q}', m, \tau, c, v\rangle$. The excitonic state with momentum $\mathbf{q}$, quantum number $n$, in the valley $\tau$, with an electron in $(c+j)$ conduction band and a hole in $(v-l)$ valence band reads

$$|\mathbf{q}, n, \tau, c+j, v-l\rangle = \frac{1}{\sqrt{S}}\int d^2\mathbf{r}_e \int d^2\mathbf{r}_h e^{i\mathbf{q}\cdot\mathbf{R}}\Phi_n^{c+j,v-l}(\mathbf{r}_e-\mathbf{r}_h)\psi^{\dagger}_{c+j,\tau}(\mathbf{r}_e)\psi_{v-l,\tau}(\mathbf{r}_h)|0\rangle. \tag{11}$$

Here $\mathbf{R} = (\mu_{c+j}\mathbf{r}_e + \mu_{v-l}\mathbf{r}_h)/(\mu_{c+j}+\mu_{v-l})$ is the coordinate of the center-of-mass of electron and hole quasiparticles with effective masses $\mu_{c+j}$ and $\mu_{v-l}$ respectively. $\mathbf{q}$ is the momentum of the exciton, $\Phi_n^{c+j,v-l}(\mathbf{r}_e-\mathbf{r}_h)$ is the wave-function of two-body problem, i.e., the relative-motion of the electron and the hole. Here we introduced the electron

$$\psi_{c+j,\tau}(\mathbf{r}_e) = \frac{1}{\sqrt{S}}\sum_{\mathbf{k}} e^{i\mathbf{k}\cdot\mathbf{r}_e}a_{\mathbf{k},c+j,\tau}, \tag{12}$$

and the hole

$$\psi_{v-l,\tau}(\mathbf{r}_h) = \frac{1}{\sqrt{S}} \sum_{\mathbf{k}} e^{i\mathbf{k}\cdot\mathbf{r}_h} a_{\mathbf{k},v-l,\tau} \tag{13}$$

annihilation operators acting in the point with the coordinate $\mathbf{r}_e$ of $(c+j)$ band and in the point with the coordinate $\mathbf{r}_h$ of the $(v-l)$ band, respectively. We consider the sample of finite area $S$, and discrete set of momentum $\mathbf{q}$ in the system, which satisfy the following completeness and orthogonality relations

$$\frac{1}{S}\sum_{\mathbf{q}} e^{i\mathbf{q}\cdot(\mathbf{r}-\mathbf{r}')} = \delta(\mathbf{r}-\mathbf{r}')), \quad \frac{1}{S}\int_S d^2\mathbf{r}\, e^{i(\mathbf{q}-\mathbf{q}')\cdot\mathbf{r}} = \delta_{\mathbf{q}\mathbf{q}'}. \tag{14}$$

Using all the aforementioned statements we conclude that the excitonic states are normalized to the unity

$$\langle \mathbf{q}, n, \tau, c+j, v-l | \mathbf{q}', n', \tau', c+j', v-l' \rangle = \delta_{\mathbf{q}\mathbf{q}'}\delta_{nn'}\delta_{\tau\tau'}\delta_{jj'}\delta_{ll'}. \tag{15}$$

Substituting the excitonic states into the Eq. (5) we obtain

$$\begin{aligned} M_{\mathbf{q}',m,\tau} =& - e^2\sqrt{S}\delta_{\mathbf{q}',\mathbf{0}}e^{i(\phi_1+\phi_2)}\times \\ &\times \sum_n \Bigg[\frac{\gamma_6\gamma_4^*}{(E_{c+2}-E_v)(E_{c+2}-E_c)}[\Phi_n^{c+2,v}(0)]^*\Big\{\int d^2\mathbf{r}\,[\Phi_m^{c,v}(\mathbf{r})]^*\Phi_n^{c+2,v}(\mathbf{r})\Big\} + \\ &\quad + \frac{\gamma_5\gamma_2^*}{(E_c-E_{v-3})(E_v-E_{v-3})}[\Phi_n^{c,v-3}(0)]^*\Big\{\int d^2\mathbf{r}\,[\Phi_m^{c,v}(\mathbf{r})]^*\Phi_n^{c,v-3}(\mathbf{r})\Big\}\Bigg] \times \\ &\quad \times \Big[\frac{1}{E_n(0)-\hbar\omega_1} + \frac{1}{E_n(0)-\hbar\omega_2}\Big], \end{aligned} \tag{16}$$

where $\phi_1 = \arccos(\mathbf{e}_1\cdot\mathbf{e}_x)$ and $\phi_2 = \arccos(\mathbf{e}_2\cdot\mathbf{e}_x)$. Since, $M_\tau \propto \exp(i\phi_1 + i\phi_2)$ and $\Gamma_{\mathbf{q}',m} \propto \sum_\tau |M_{\mathbf{q}',m,\tau}|^2$, we conclude that, the absorption coefficient doesn't demonstrate any dependence on the polarizations of the pump and probe pulses. Finally, the absorption amplitude doesn't depend on the valley index. Note that the only transitions from the

ground states to the intermediate $s$ excitonic states give a contribution to the amplitude, because $\Phi_n^{c+j,v-l}(0) \neq 0$ only for $n = 1s, 2s, \dots$ states. Therefore, the integrals in braces are non-zero only if the final excitonic wave-function $\Phi_m^{c,v}(\mathbf{r})$ is also $s$ state, due to orthogonality of the states with the different angular momentums. The shape of $s$ states of all three wave functions are different. However, as a first approximation we can suppose that that the ovelapping integrals dominates only for $m = n$ case, i.e., we suppose

$$\int d^2\mathbf{r}\,[\Phi_m^{c,v}(\mathbf{r})]^*\Phi_n^{c+2,v}(\mathbf{r}) \approx \int d^2\mathbf{r}\,[\Phi_m^{c,v}(\mathbf{r})]^*\Phi_n^{c,v-3}(\mathbf{r}) \approx \delta_{nm}. \quad (17)$$

Such an approximation provides the following approximate result

$$|M_{\mathbf{q}',m,\tau}| \approx -e^2\sqrt{S}\delta_{\mathbf{q}',\mathbf{0}}\left[\frac{\gamma_6\gamma_4^*\Phi_m^{c+2,v}(0)}{(E_{c+2}-E_v)(E_{c+2}-E_c)} + \frac{\gamma_5\gamma_2^*\Phi_m^{c,v-3}(0)}{(E_c-E_{v-3})(E_v-E_{v-3})}\right]\times \quad (18)$$

$$\times\sum_{j=1}^{2}\frac{1}{E_m(0)-\hbar\omega_j}. \quad (19)$$

Substituting this result into Eq. (4) we calculate the total absorption rate of photons' energy per unit area

$$\frac{\partial W}{\partial t} = -\sum_{\mathbf{q}',m} E_m(\mathbf{q}')\Gamma_{\mathbf{q}',m} = -\Big(\frac{c}{8\pi}|E_1|^2\Big)\Big(\frac{c}{8\pi}|E_2|^2\Big)\beta(\omega_1,\omega_2) = -I_1I_2\beta(\omega_1,\omega_2), \quad (20)$$

where $I_1$ and $I_2$ are the intensities of the first and the second pulses, respectively, and

$$\beta(\omega_1,\omega_2) = 256\pi^3\alpha^2\hbar\sum_m\left[\frac{\gamma_6\gamma_4^*\Phi_m^{c+2,v}(0)}{(E_{c+2}-E_v)(E_{c+2}-E_c)} + \frac{\gamma_5\gamma_2^*\Phi_m^{c,v-3}(0)}{(E_c-E_{v-3})(E_v-E_{v-3})}\right]^2\times$$
$$\times\left[\frac{1}{E_m(0)-\hbar\omega_1} + \frac{1}{E_m(0)-\hbar\omega_2}\right]^2 E_m(0)\delta(E_m(0)-\hbar\omega_1-\hbar\omega_2). \quad (21)$$

where $\alpha = e^2/\hbar c$ is the fine structure constant. Comparing the parameters of Eq. (20) with the similar equation for bulk crystals (see Ref. [9]) we conclude that the parameter $\beta(\omega_1,\omega_2)$ can

be associated with the absorption coefficient for the monolayer TMD. To evaluate the numerical value of this coefficient one needs to know: the $\mathbf{k}\cdot\mathbf{p}$ coupling parameters $\gamma_2, \gamma_4, \gamma_5, \gamma_6$, the energies $E_{v-3}, E_v, E_c, E_{c+2}$ (see Ref.[10]); numerical values of $\Phi_m^{c+2,v}(\mathbf{r})$ and $\Psi_m^{c,v-3}(\mathbf{r})$ of $m = 1s, 2s, \ldots$ exciton wave functions at $\mathbf{r} = 0$, which can be evaluated numerically using $\mathbf{k}\cdot\mathbf{p}$ parameters[10] and the two-body approximation (see Supplementary data in[11]); and the spectrum of excitons $E_m(0)$ in monolayer TMD.[12]

Using the properties of the delta function we rewrite the expression for the absorption coefficient in the form

$$\beta(\omega_1,\omega_2) = 256\pi^3\alpha^2\frac{(\omega_1+\omega_2)^3}{\omega_1^2\omega_2^2}\sum_m\left[\frac{\gamma_6\gamma_4^*\Phi_m^{c+2,v}(0)}{(E_{c+2}-E_v)(E_{c+2}-E_c)} + \frac{\gamma_5\gamma_2^*\Phi_m^{c,v-3}(0)}{(E_c-E_{v-3})(E_v-E_{v-3})}\right]^2 \times \tag{22}$$

$$\times\, \delta(E_m(0) - \hbar\omega_1 - \hbar\omega_2). \tag{23}$$

During the derivation of the formula we did not take into account the processes which can lead to the broadening of the exciton lines. We modify the corresponding formula by introducing the phenomenological broadening parameter $\Gamma$ by replacing

$$\delta(E_m(0) - \hbar\omega_1 - \hbar\omega_2) \to \frac{1}{\pi}\mathrm{Im}\Big[\frac{1}{E_m(0) - \hbar\omega_1 - \hbar\omega_2 - i\Gamma}\Big], \tag{24}$$

in the Eq. (22). Note that this result is applicable only if the photon energies $\hbar\omega_1, \hbar\omega_2 < E_m(0) - \Gamma$, i.e. both energies should be far from the resonance energies $E_m(0)$.

The functions $\Phi_m^{c+2,v}(0)$ and $\Phi_m^{c,v-3}(0)$ decay significantly with the principal number $m$ of the state. In the case of the hydrogen atom the corresponding behavior is $\propto 1/(m-1/2)^{3/2}$. Note that this behavior is $\propto 1/(m+\delta)^2$ for the case of the TMD monolayers, where the parameter $\delta \sim 0$ is called the excitonic quantum defect, see details in.[12] Therefore the general contribution to the absorption coefficient appears from $m = 1\ s$ excitonic state,

which gives the corresponding approximate result

$$\beta(\omega_1,\omega_2) = 256\pi^3\alpha^2\hbar\frac{(\hbar\omega_1+\hbar\omega_2)^3}{(\hbar\omega_1)^2(\hbar\omega_2)^2}\left[\frac{\gamma_6\gamma_4^*\Phi_{1s}^{c+2,v}(0)}{(E_{c+2}-E_v)(E_{c+2}-E_c)}+\frac{\gamma_5\gamma_2^*\Phi_{1s}^{c,v-3}(0)}{(E_c-E_{v-3})(E_v-E_{v-3})}\right]^2\times$$
$$\times\,\delta(E_{1s}(0)-\hbar\omega_1-\hbar\omega_2)\propto\frac{(\hbar\omega_1+\hbar\omega_2)^3}{(\hbar\omega_1)^2(\hbar\omega_2)^2}\frac{\Gamma}{(E_{1s}(0)-\hbar\omega_1-\hbar\omega_2)^2+\Gamma^2}. \quad (25)$$

For the fixed value of the pump frequency $\omega_1$ the formula provides the asymmetric shape of the absorption coefficient as a function of remaining frequency $\omega_2$. The corresponding function, for the experimental values of A-and B excitons $E_{1s}^A(0)\approx 1.886$ eV and $E_{1s}^B(0)\approx 2.032$ eV, respectively, $\Gamma\approx 26$ meV, $\hbar\omega_1\approx 0.62$ eV, as a function of the energy parameter $\hbar\omega_2$. The sketch of the absorption coefficient is presented in Supplementary Fig. 1a.

In order to estimate the absorption coefficient in the energy domain beyond the $1s$ exction resonance we need to take into account the $m$ dependence of $\Phi_m^{c+2,v}(0)$ and $\Phi_m^{c,v-3}(0)$ parameters. Using the result of Ref.[12] we can approximately write $\Phi_m^{c+2,v}(0)\approx A/(m+\delta_1)^2$, $\Phi_{1s}^{c,v-3}(0)\approx B/(m+\delta_2)^2$, and $\Phi_m^{c,v}(0)\propto C/(m+\delta)^2$. The excitonic quantum defect parameters $\delta_1$, $\delta_2$ and $\delta$ depend on the reduced mass of the excitons $\mu^{c+2,v}$, $\mu^{c,v-3}$, and $\mu$ respectively. In order to proceed further with the calculation we assume roughly $\delta_1=\delta_2=\delta$ (the general case can also be calculated but with providing a more bulky result). It is slightly change the amplitudes of the absorption peaks but not their positions. Using this approximation we modify the Eq. (22) and present it into form of the Elliott formula

$$\beta(\omega_1,\omega_2) \approx 256\pi^3\alpha^2\frac{(\omega_1+\omega_2)^3}{\omega_1^2\omega_2^2}\left[\frac{\gamma_6\gamma_4^*A}{(E_{c+2}-E_v)(E_{c+2}-E_c)}+\frac{\gamma_5\gamma_2^*B}{(E_c-E_{v-3})(E_v-E_{v-3})}\right]^2\times$$
$$\times\sum_{m=1}^{\infty}\frac{1}{(m+\delta)^4}\delta(E_m(0)-\hbar\omega_1-\hbar\omega_2). \quad (26)$$

To estimate the absorption coefficient we can use the semi-analytical formula for the

spectrum of the excitons[12]

$$E_m(0) = E_g - Ry^* \frac{\gamma}{(m+\delta)^2}, \tag{27}$$

where $E_g$ is the single-particle band gap in the system, $Ry^* = \mu e^4/(2\hbar^2\varepsilon^2)$ is the effective Rydberg energy, for the exciton with reduced mass $\mu$ and dielectric constant $\varepsilon$ of the medium surrounded the monolayer. Dimensionless parameters $\gamma, \delta$ depend on the ratio of the effective Bohr radius $a_0^* = \hbar\varepsilon/m_0 e^2$ and effective in-plane screening length of the monolayer $r_0^* = r_0/\varepsilon$. Taking into account the parameters for the considered system $\varepsilon = 1.6$, $\mu = 0.26m_0$, $r_0 = 41.5$Å, the energy positions of the $1s$ states for $A$ and $B$ excitons $E_{1s}^A = 1.886$ meV and $E_{1s}^B = 2.032$ meV, respectively[8] we obtain $Ry^* \approx 1.38$ eV, $\gamma \approx 0.943$, $\delta \approx 0.746$. Using these parameters we calculate the spectrum of the excitons. Then using the Elliott type formula we estimate the absorption coefficient for the first 5 $s$ excitonic states and broadened delta function with $\Gamma = 0.026$ eV and present it in Supplementary Fig. 1b and in the Fig. 4b in the main text.

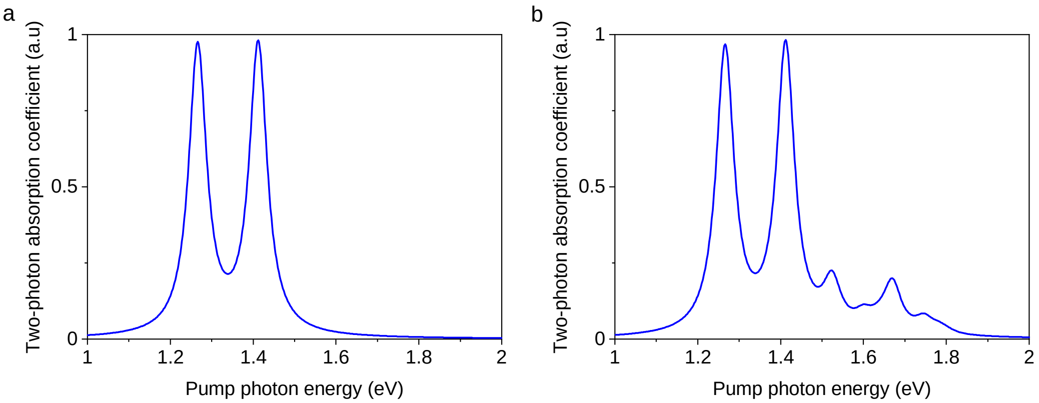


Supplementary Figure 1: Two-photon absorption coefficient $\beta(\omega_1, \omega_2)$ calculated using Eq. (26) as a function of the photon energy $\hbar\omega_2$ with the photon energy of the first wave fixed at $\hbar\omega_1 = 0.62$ eV. (a) The spectra calculated only with the lowest 1sA and 1sB exciton states. (b) The spectra obtained with the lowest 5 $s$ A and B exciton states.

# References

(1) Kormányos, A.; Burkard, G.; Gmitra, M.; Fabian, J.; Zólyomi, V.; Drummond, N. D.; Fal'ko, V. k· p theory for two-dimensional transition metal dichalcogenide semiconductors. *2D Mater.* **2015**, *2*, 022001.

(2) Liu, G.-B.; Xiao, D.; Yao, Y.; Xu, X.; Yao, W. Electronic structures and theoretical modelling of two-dimensional group-VIB transition metal dichalcogenides. *Chem. Soc. Rev.* **2015**, *44*, 2643–2663.

(3) Wang, G.; Bouet, L.; Glazov, M.; Amand, T.; Ivchenko, E.; Palleau, E.; Marie, X.; Urbaszek, B. Magneto-optics in transition metal diselenide monolayers. *2D Mater.* **2015**, *2*, 034002.

(4) Kormányos, A.; Zólyomi, V.; Drummond, N. D.; Burkard, G. Spin-orbit coupling, quantum dots, and qubits in monolayer transition metal dichalcogenides. *Phys. Rev. X* **2014**, *4*, 011034.

(5) Glazov, M. M.; Golub, L. E.; Wang, G.; Marie, X.; Amand, T.; Urbaszek, B. Intrinsic exciton-state mixing and nonlinear optical properties in transition metal dichalcogenide monolayers. *Phys. Rev. B* **2017**, *95*, 035311.

(6) Landau, L. D.; Lifshitz, *Quantum mechanics: non-relativistic theory*; Butterworth-Heinemann, 1981; Vol. 3.

(7) Sakurai, J. J.; Commins, E. D. Modern quantum mechanics. 2020.

(8) Slobodeniuk, A.; Koutenský, P.; Bartoš, M.; Troják, F.; Malý, P.; Novotný, T.; Kozák, M. Semiconductor Bloch equation analysis of optical Stark and Bloch-Siegert shifts in monolayer $WSe_2$ and $MoS_2$. *Phys. Rev. B* **2022**, *106*, 235304.

(9) Bass, M.; Van Stryland, E. W.; Williams, D. R.; Wolfe, W. L. *Handbook of optics*; McGraw-Hill Professional, 1994; Vol. 1.

(10) Rybkovskiy, D. V.; Gerber, I. C.; Durnev, M. V. Atomically inspired k·p approach and valley Zeeman effect in transition metal dichalcogenide monolayers. *Phys. Rev. B* **2017**, *95*, 155406.

(11) Kipczak, Ł.; Slobodeniuk, A. O.; Woźniak, T.; Bhatnagar, M.; Zawadzka, N.; Olkowska-Pucko, K.; Grzeszczyk, M.; Watanabe, K.; Taniguchi, T.; Babiński, A., et al. Analogy and dissimilarity of excitons in monolayer and bilayer of $MoSe_2$. *2D Mater.* **2023**, *10*, 025014.

(12) Molas, M.; Slobodeniuk, A.; Nogajewski, K.; Bartos, M.; Babiński, A.; Watanabe, K.; Taniguchi, T.; Faugeras, C.; Potemski, M., et al. Energy spectrum of two-dimensional excitons in a nonuniform dielectric medium. *Phys. Rev. Lett.* **2019**, *123*, 136801.
